# Supplementary material for: Cooperative Relative Localization in MAV Swarms with Ultra-wideband Ranging
Source: arXiv:2405.18234 source file (2024-05-28)
Supplement: Supplementary file 2 [file appendix2-proof.tex]

\section{Proof2}
